# Supplementary material for: SpatialCoT: Advancing Spatial Reasoning through Coordinate Alignment and Chain-of-Thought for Embodied Task Planning
Source: arXiv:2501.10074 source file (2025-01-23)
Supplement: Supplementary file 1 [file training_details.tex]

\begin{table}[]
\centering
\begin{tabular}{c|c}
\hline
\textbf{Hyperparameters} & \textbf{Value} \\ \hline
learning\_rate & 1e-5 \\ \hline
learning\_rate\_decay (per epoch) & 0.9 \\ \hline
weight\_decay & 0 \\ \hline
gradient\_clipping & False \\ \hline
batch\_size & $16\times8$ \\ \hline
batching\_strategy & padding \\ \hline
num\_epochs & 3 \\ \hline
peft\_method & lora \\ \hline
freeze\_layers & False \\ \hline
enable\_fsdp & True \\ \hline
\end{tabular}
\label{tab:hyperparameters}
\title{Hyper-parameters for Model Training}
\end{table}
